# Supplementary material for: Excretion Detection in Pigsties Using Convolutional and Transformerbased Deep Neural Networks
Source: arXiv:2412.00256 source file (2026-04-22)
Supplement: Supplementary file 1 [file Appendix_1.tex]

\section{Schematic representation of the architectures described in \autoref{subsec:models}}
\label{appendix:A}

\begin{figure}[h]
  \centering
  \includegraphics[width=\linewidth]{Figures/Faster_R-CNN.png}
  \caption[Architecture of a Faster \ac{r-cnn}]{Main components of the architecture of a Faster \ac{r-cnn} according to \citep{Software_Faster_R-CNN}}
  \label{fig:Faster_R-CNN}
\end{figure}

\begin{figure}[h]
  \centering
  \includegraphics[width=\linewidth]{Figures/YOLO_v8.png}
  \caption[Architecture of a \ac{yolo}v8.]{Main components of the architecture of a \ac{yolo}v8.}
  \label{fig:YOLO_v8}
\end{figure}

\begin{figure}[h]
  \centering
  \includegraphics[width=\linewidth]{Figures/DETR.png}
  \caption[Architecture of a \ac{detr}.]{Illustration of the \ac{detr} architecture with encoder and decoder}.
  \label{fig:DETR}
\end{figure}

\begin{figure}[h]
  \centering
  \includegraphics[width=\linewidth]{Figures/DAB-DETR.png}
  \caption[Architecture of a \ac{dab-detr}.]{Architecture of a \ac{dab-detr} with entire anchor boxes instead of position coding}
  \label{fig:DAB-DETR}
\end{figure}
